# Supplementary material for: Infrared study of the spin reorientation transition and its reversal in the superconducting state in underdoped Ba$ _{1-x} $K$ _{x} $Fe$ _{2} $As$ _{2} $
Source: arXiv:1505.01645 source file (2015-05-07)
Supplement: Supplementary file 1 [file Mallett__BKFAoptics_tAFphase_SOM.pdf]

# Supplementary information: Infrared study of the spin reorientation transition and its reversal in the superconducting state in underdoped $Ba_{1-x}K_xFe_2As_2$

B.P.P. Mallett,[1] P. Marsik,[1] M. Yazdi-Rizi,[1] Th. Wolf,[2] A.E. Böhmer,[2] F. Hardy,[2] C. Meingast,[2] D. Munzar,[3] and C. Bernhard[1]

[1] *University of Fribourg, Department of Physics and Fribourg Center for Nanomaterials, Chemin du Muse 3, CH-1700 Fribourg, Switzerland*

[2] *Karlsruhe Institute of Technology, Postfach 3640, Karlsruhe 76021, Germany*

[3] *Department of Condensed Matter Physics, Faculty of Science and Central European Institute of Technology, Masaryk University, Kotlářska 2, 61137 Brno, Czech Republic*

(Dated: April 30, 2015)

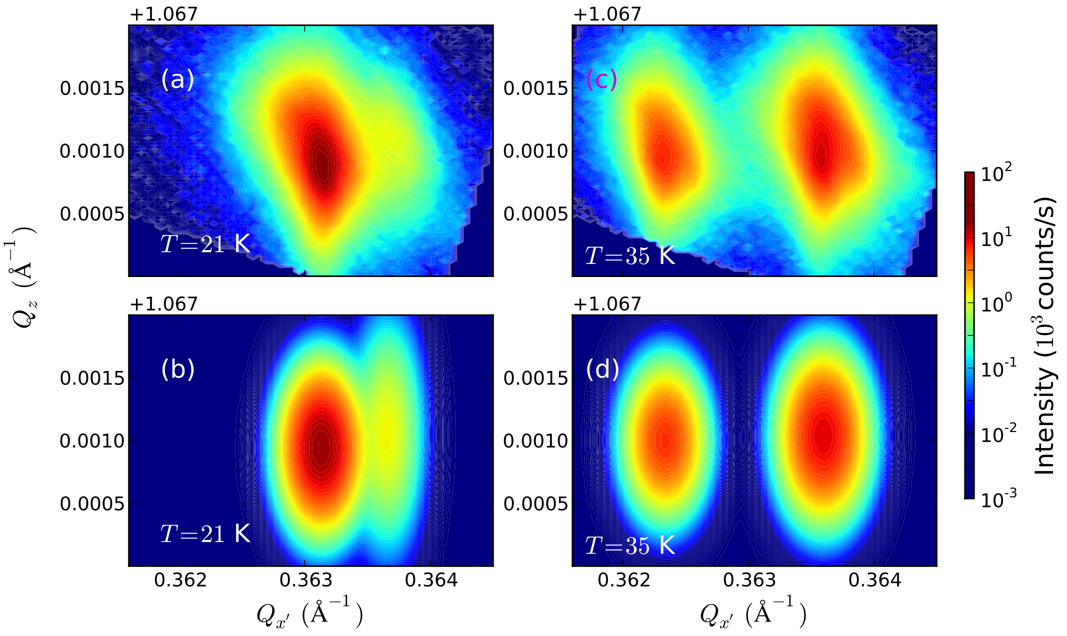


FIG. 1. (a) X-ray diffractometry data at $T = 21$ K (in the t-AF phase) in a region of reciprocal space around the $(1, 1, 14)$ Bragg peak. Note the log scale. Panel (b) shows a fit to the $T = 21$ K data. Panels (c) and (d) show the data and fit at $T = 35$ K (in the o-AF phase), respectively.

## X-RAY DIFFRACTION DATA

In the high-temperature tetragonal phase above $T^{\mathrm{N1}}$, $\mathrm{Ba}_{1-x}\mathrm{K}_x\mathrm{Fe}_2\mathrm{As}_2$ has the space group $I4/mmm$. As the temperature is lowered, the tetragonal $(1, 1, 14)$ Bragg-peak is known to split into two peaks below the tetragonal to orthorhombic structural transition. Below we denote the distance in reciprocal space in the $(1, 1, 0)$ direction as $Q_{x'}$. This splitting of the Bragg peak in the $Q_{x'}$ direction we observe with x-ray diffraction, as shown in Fig. 1(a) of the main paper and in Fig. S1(c). In the t-AF phase between $T^{\mathrm{N2}}$ and $T^{\mathrm{N3}}$, the intensity of these split orthorhombic peaks decreases strongly whilst a third Bragg-peak at intermediate $Q_{x'}$ grows in intensity. This is shown in Fig. S1(a) which plots the diffracted x-ray intensity in a region of reciprocal space around the $(1, 1, 14)$ Bragg-peak in the t-AF phase at $T = 21$ K. The main feature is this Bragg-peak at intermediate $Q_{x'} = 0.3631$ Å$^{-1}$ whilst only a weak remnant of one of the split orthorhombic peaks can be seen at larger $Q_{x'}$. This demonstrates that the majority of the sample is tetragonal (or has an orthorhombic splitting smaller than our experimental resolution) in the t-AF phase.

In order to estimate what fraction of the sample remains with this orthorhombic symmetry

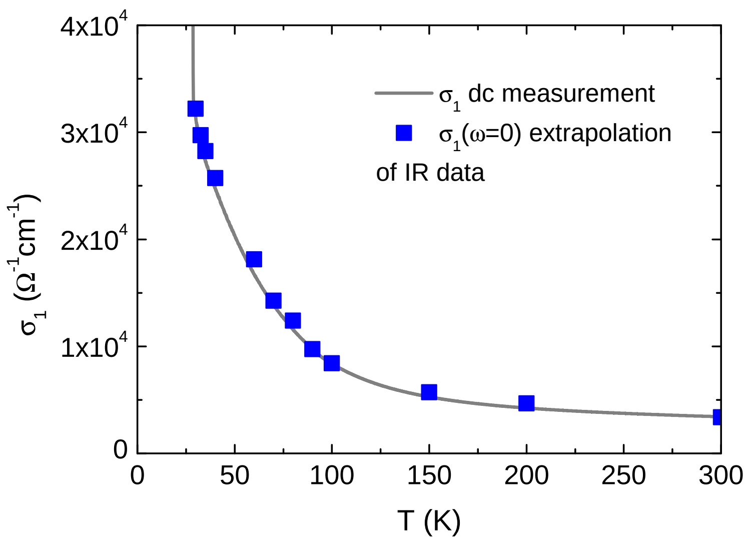


FIG. 2. The measured dc conductivity (solid line) and the extrapolated values of the optical conductivity at $\omega = 0$ (squares).

in the t-AF phase, each of the three Bragg peaks were fitted to an asymmetric 2-dimensional Gaussian function;

$$I = A\exp\left[-\frac{(Q_{x'}-\mu_{x'})^2}{2\sigma_{x'}^2} - \frac{(Q_z-\mu_z)^2}{2\sigma_z^2}\right]$$

The volume of this function is $2\pi A\sigma_{x'}\sigma_z$, which we call here the weight. From the fit shown in Fig. S1(b) we find that in the t-AF phase, the weight of the one observable orthorhombic peak is 10(1)% the weight of the main tetragonal peak. It is also 10(1)% of the combined weight of the two orthorhombic Bragg reflections in the o-AF phase.

## LOW-FREQUENCY EXTRAPOLATION OF THE OPTICAL CONDUCTIVITY

In the normal-state, the optical conductivity was extrapolated to zero-frequency by fitting two Drude terms (and several higher-frequency Lorentz terms) to the FIR reflectivity and MIR ellipsometry data. The use of two Drude terms in fitting the optical conductivity data in the pnictides has been discussed at length in the literature, see [1, 2] and references therein. Fig. S2 shows the extrapolated $\sigma_1(\omega = 0)$ values from the optics data against the DC conductivity measured by the conventional 4-probe technique.

In the superconducting state below $T = 28$ K, the low-frequency extrapolation of the reflectivity data was achieved using the so-called gapped Drude model and implemented in

the RefFIT program written by Alexey Kuzmenko [3]. These extrapolations, shown as dotted lines in Fig. 2(b), were then used in the determination of the superconducting condensate density, $\omega_{pl,SC}^2 \propto n_s$ , where the reduction of the spectral-weight over the spectral range $0^+$ to 2000 cm$^{-1}$ below $T_c$ with respect to $T > T_c$ is taken to be equal to $\omega_{pl,SC}^2$. As stated in the main text, the accuracy of these extrapolations was checked against estimates of $\omega_{pl,SC}^2$ utilizing the real part of the dielectric function, $\epsilon_1$. The contribution to $\epsilon_1$ for a Drude term with zero scattering rate (representing SC charge-carriers) is $\epsilon_{1,\delta} = 1 - \omega_{pl}^2/\omega^2$, where the plasma frequency $\omega_{pl} = 2e\sqrt{\pi n/m^*}$ is related to the charge-carrier density, $n$, and effective-mass, $m^*$. However, the measured $\epsilon_1$ also contains additional contributions from finite-frequency oscillators which must be accounted for in order to estimate the plasma frequency of the superconducting condensate, $\omega_{pl,SC}$. This is achieved by taking the Kramers-Kronig transformation of the measured $\sigma_1(\omega)$ in the range $0^+ < \omega < 4000$ cm$^{-1}$ (or, equivalently, of $\epsilon_2(\omega)$ since $\sigma(\omega) = \frac{i\omega}{4\pi}[1 - \epsilon(\omega)]$) which yields a function, $\epsilon_1^{reg}(\omega)$, that would be measured in the absence of a superconducting condensate. One then obtains an upper estimate of $\omega_{pl,SC}$ by equating $\epsilon_{1,\delta}$ with $\epsilon_1 - \epsilon_1^{reg}$. The two methods give similar values of $\omega_{pl,SC}$ across the entire temperature range and in Fig. 3(e) of the main text we show an average of $\omega_{pl,SC}^2$ from these two methods at each temperature and indicate the difference between the two methods in the error bars.

## SPECTRAL WEIGHT OF THE SDW PAIR-BREAKING PEAK

In an itinerant magnetic model, the spectral-weight (SW) of the pair-breaking peak is proportional to the magnitude of the AF moments. To estimate the SW of the pair-breaking peak, we firstly fit the 'normal state' (i.e. $T > T^{\mathrm{N1}}$) $\sigma(\omega) = \sigma_1(\omega) + i\sigma_2(\omega)$ data between 0 and 4000 cm$^{-1}$ using two Drude terms and three broad Lorentzian oscillators. Such a fit is shown in Fig. S3(a) for our underdoped crystal at 100 K. Fitting the $\sigma(\omega)$ data below $T^{\mathrm{N1}}$, we keep the Lorentzian oscillators fitted from the data above $T^{\mathrm{N1}}$ essentially fixed (allowing only for small changes of the oscillator strength). The remainder of the spectra are fitted by varying the Drude terms and introducing Gaussian oscillators to fit the pair-breaking peak. Gaussian oscillators are used because they are more localized than Lorentz oscillators and still give a phenomenological description of the data. The SW, $\int \sigma_1(\omega)d\omega$, of the pair-breaking peak is then determined from the fitted Gaussian oscillators.

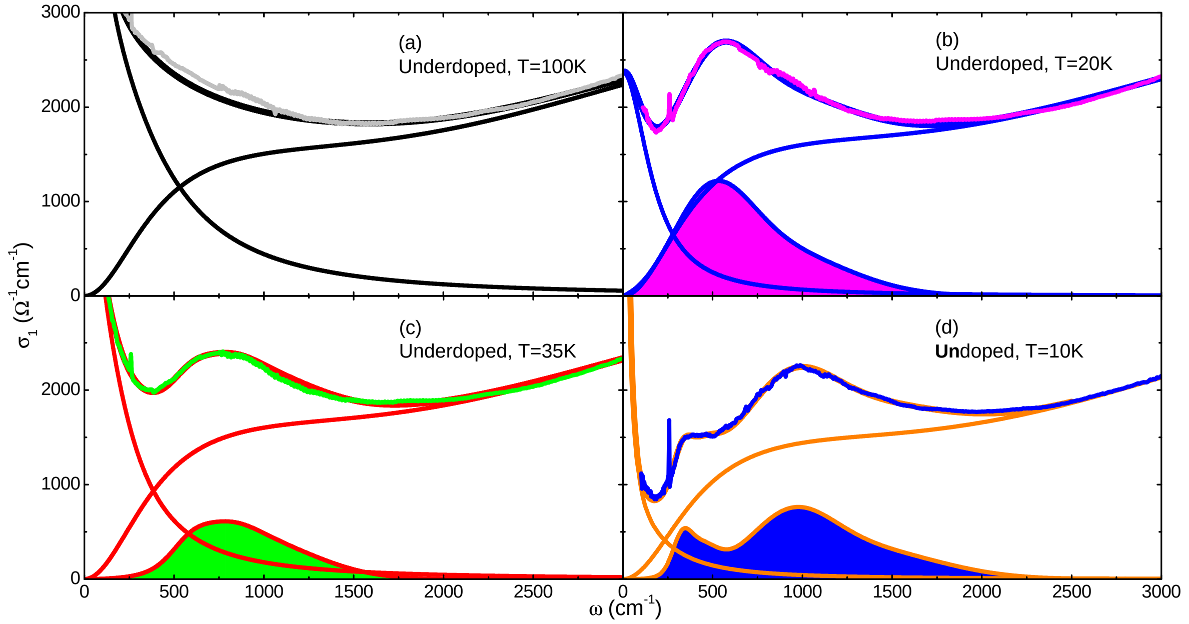


FIG. 3. (a) $\sigma_1(\omega)$ at 100 K ($T > T^{\mathrm{N1}}$) for our underdoped crystal showing the fitted Drude-Lorentz oscillators. (b) The pair-breaking peak in $\sigma_1(\omega)$ in the t-AF phase at 20 K, (c) in the o-AF phase at 35 K and (d) for the parent compound, $BaFe_2As_2$, at 10K. In each spectrum, this feature is fitted to a sum of Gaussian oscillators, shown shaded. The background from the broad Lorentz oscillators is kept essentially fixed from the $T > T^{\mathrm{N1}}$ fits.

We consider three spectra; our underdoped crystal at 20 and 35 K representing typical SDW weights in the t-AF and o-AF phases respectively, and the parent compound (K=0%) at $T = 10$ K from Marsik *et al.* [4]. These data are shown in Fig. S3(b), (c) and (d) respectively. The fitted pair-breaking-peak features are shown as shaded curves with the backgrounds and overall fits shown as lines. From these we obtain the following SWs of the pair-breaking peaks; (9.1, 4.6 and 7.6)$\times 10^5$ $\Omega^{-1}\mathrm{cm}^{-2}$ for our underdoped crystal at $T = 20$ and 35 K and the parent compound at 10 K respectively.

## PHONONS

Finally, we have suggested that the main component of the satellite of the IR-active mode at 259 $\mathrm{cm}^{-1}$ in the t-AF phase can be attributed to a specific out-of-phase iron mode. As noted in the main text, a likely spin-structure of the t-AF phase is that shown in Fig.4 of Ref. [5] which is reproduced here in Fig. S4(a) (for clarity, only the Fe sites are shown). The

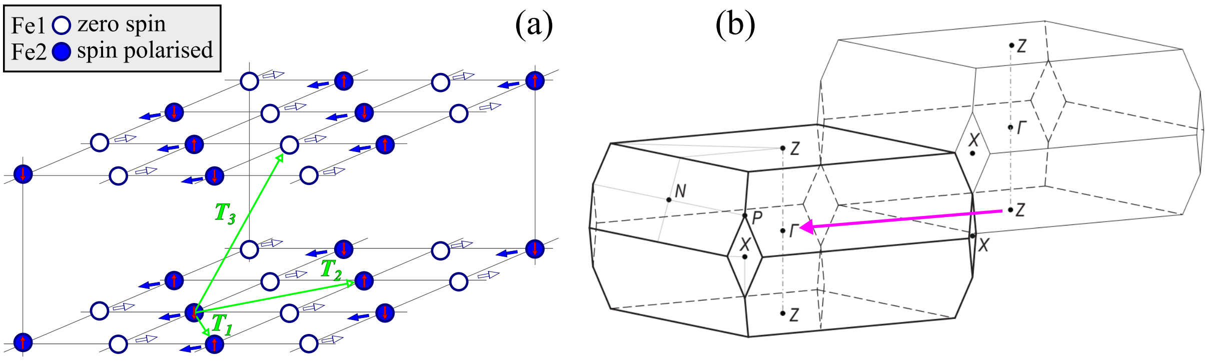


FIG. 4. Configuration of the spin-structure as in the t-AF phase as in Fig. 4 of Ref. [5]. For clarity, only the Fe sites are shown. The symbols $T_1$, $T_2$ and $T_3$ indicate the primitive translations for the parent body-centered tetragonal lattice [6]. Ionic displacements for the out-of-phase iron mode are indicated by the blue/white arrows. Panel (b) Two neighboring Brillouin zones of the body-centered tetragonal lattice, reproduced from Ref. [6]. The arrow indicates the relevant folding.

ionic displacements corresponding to the out-of-phase iron mode are indicated by blue/white arrows. From the point of view of the parent body-centered tetragonal (bct) structure, this is a $Z$-point mode. This mode is normally not IR active (the related $\Gamma$ mode, the one with the highest frequency where the ions connected by $T_3$ vibrate in-phase, is Raman active [7]). However, it becomes a $\Gamma$ point IR active mode in the t-AF phase due to the inequivalence of the Fe1 and Fe2 sites. The oscillator strength of the mode is determined by the difference between the dynamical effective charges of Fe1 and Fe2. Fig. S4(b) shows the first Brillouin zone (BZ) of the bct lattice and a neighboring BZ (reproduced from Ref. [6], Fig.10). The pink arrow shows the folding of the $Z$-point of the BZ of the bct lattice to the BZ of the t-AF phase.

---


[1] A. Charnukha, Journal of Physics: Condensed Matter **26**, 253203 (2014).

[2] P. Marsik, C. N. Wang, M. Rössle, M. Yazdi-Rizi, R. Schuster, K. W. Kim, A. Dubroka, D. Munzar, T. Wolf, X. H. Chen, and C. Bernhard, Phys. Rev. B **88**, 180508 (2013).

[3] A. Kuzmenko, "Reffit," .

[4] P. Marsik, C. N. Wang, M. Rössle, M. Yazdi-Rizi, R. Schuster, K. W. Kim, A. Dubroka, D. Munzar, T. Wolf, X. H. Chen, and C. Bernhard, Phys. Rev. B **88**, 180508 (2013).

[5] D. D. Khalyavin, S. W. Lovesey, P. Manuel, F. Krüger, S. Rosenkranz, J. M. Allred, O. Chmaissem, and R. Osborn, Phys. Rev. B **90**, 174511 (2014).

[6] O. Andersen and L. Boeri, Annalen der Physik **523**, 8 (2011).

[7] M. Sandoghchi, H. Khosroabadi, H. Almasi, and M. Akhavan, Journal of Superconductivity and Novel Magnetism **26**, 93 (2013).
